# Supplementary material for: Automated Quantum Software Engineering: why? what? how?
Source: arXiv:2212.00619 source file (2022-12-01)
Supplement: Supplementary file 1 [file appendix_1.tex]

\newpage

\section{Background}

\subsection{Resource theories for quantum computation}

\begin{figure}[bht]
\centering %LBRT
\includegraphics[clip, trim=0cm 2cm 0cm 2cm,width=0.99\textwidth]{figures/AQSE.pdf}
\caption{Main blocks and workflow for Automated Quantum Software Engineering}
\label{fig:aqse}
\end{figure}

Considerations:
\begin{itemize}[nolistsep,noitemsep]
    \item how much distinguishability is needed to identify the solution from the non-solutions (e.g. if the statistics of measurement results is tipped 51-49, can I conclude that the solution is the first state?)
    \item how long a coherence time or noise level is permissible for the given distinguisability ofr the specific algorithm?
    \item how many qubits are there in the hardware (can be generalized to qudits)?
    \item how are the qubits connected?
    \item what are the noise characteristics of each qubits and each pair of 2-qubits?
    \item what is the connectivity topology of the QPU?
    \item how many extra gates are needed to map the program to this connectivity topology?
    \item what are the native gateset and the best way to convert the gates in the algorithm to these?
    \item given the topology, noise model and gateset, what quantum error correction code would provide an advantage and how to implement it?
\end{itemize}

It is not surprising that most of these considerations are fairly low level.
As with current high-level classical programming, or even classical assembly/hdl level programming, we expect these to be abstracted from the quantum algorithm designer as part of the quantum accelerator and compiler layer.
Nevertheless, even in a hardware-agnostic approach, it is beneficial to consider optimizing over the number of qubits, number of gates (over any arbitrarily chosen gate-set) and increasing the solution probability (this falls more under FR and we leave this to the discussion there).

Optimizing the so-called space-time complexity of the algorithm in a fully--connected no-noise setting will very likely retail its benefit when further hardware constraints are incorporated.

\subsection{Categorical framework}

what is category theory? - objects, morphisms, axioms

why it was invented?

similarities and differences with Generalized Algebraic theory

many things can be described with many things, a figure

why then category theory - it acts as a bridge between the abstract (mind, model) and the concrete (matter, implementation)

this motivates our choice of a CT framework

success of cat theory in foundational math, and curry-howard-lambek correspondence

rosetta stone and applied cat theory, "study" other sciences from cat lens, pros of it in bridging disciplines and cross-pollination of theories/methods

applied sciences, computational category theory, from understanding to doing. examples like Lambek, catlab, hyperon

some approaches are currently trying to standardise such a framework,

\subsection{Formal Logic}

\textbf{Zeroth-order logic}: alternatively called, propositional/statement logic, sentential calculus/logic, deals with propositions, which can be either true or false.
Compound propositions are formed by connecting propositions by logical connectives. 
Propositions that contain no logical connectives are called atomic propositions.
Construction of arguments are based on relations between propositions. 
Some examples of logical connectives are $\texttt{AND}$ (conjunction, denoted by $\wedge$), $\texttt{OR}$ (disjunction, denoted by $\vee$), $\texttt{NOT}$ (negation, denoted by $\neg$) and $\texttt{IF}$ (conditional, denoted by $\rightarrow$).
In Boolean circuits, we are concerned mostly with this form of logic.

\vspace{0.7em}

\noindent\textbf{First-order logic}: Predicate logic combines the distinctive features of syllogistic logic and propositional logic.

Convert to CNF to use in circuits with universal quantifier as function oracles
% https://en.wikipedia.org/wiki/Conjunctive_normal_form#Converting_from_first-order_logic

\vspace{0.7em}

\noindent\textbf{Higher-order logic}: (short definition, and that any n-th order logic cannot be expressed in n-1 order logic).

\subsection{Learning Theory}

Q PAC

\subsection{V\&V}

Verification is a process of determining if the software is designed and developed as per the specified requirements. 

Validation is the process of checking if the software (end product) has met the client's true needs and expectations.

\subsection{Program Synthesis}

Program Synthesis is the task of automatically finding programs from the underlying programming language that satisfy user intent expressed in some form of constraints.

Difference with compiler: compilers translate between fully specified code (typically from high to low level language). 

Inputs to Program Synthesis are less specified. They search for a full-specification based on a variety of constraints (e.g. input-output examples, demonstrations, natural language, partial programs, and assertions).

2 types
\begin{itemize}[nolistsep,noitemsep]

    \item Enumerative: brute-force in some order. Effective. Enumerative search can be seen as finding a programmatic path (within an underlying grammar that connects inputs and outputs) starting from the inputs to outputs. (Con: doesn't scale well).
    
    \item Deductive synthesis: automated theorem provers construct a proof of user specification. The proof is then translated into a logical program. it searches for the programmatic path in a backward direction starting from the outputs leveraging the operator inverses. (Con: exhaustive proof search is undecidable and intractable; complete formal specification of user intent is as complicated as writing the program)
    
    \item Transformation-based synthesis: high-level specifications gradually translated to low-level. (Con: same as a compiler?)

    \item Constraint based: constraint generation and resolution. 
    
    \item Inductive synthesis: approaches like input-output examples, demonstrations, evolving programs using genetic programming, programming by example, counter-example guided. (Con: overfit vs underfit dichotomy)

    \item stochastic search: syntax guided, GP, neural program synthesis. neuroevolution?
\end{itemize}

Modern synthesizers use a combination of skeleton/grammar and specifications. The grammar provides structure to constrict the search space to the intended domain and keep the programs interpretable. 

aritra verdict: AGI needs OEE and interactions. RL-based inductive Prog.synthesis. is promising. (search process). What about search domain and user constraint specification language.

spec. language: logical specification, examples, traces, natural language, partial programs, unoptimized programs, or even related programs.

aritra verdict: probabilistic logic, input/output examples (as in AIXI), ...good. Traces in bad (too transparent) 

search space: balance between expressivity (generalization) and efficiency (tractable search).

% https://en.wikipedia.org/wiki/Superoptimization

Superoptimization is the process where a compiler automatically finds the optimal sequence for a loop-free sequence of instructions. Real-world compilers generally cannot produce genuinely optimal code, and while most standard compiler optimizations only improve code partly, a superoptimizer's goal is to find the optimal sequence, the canonical form.

% automated programming
program synthesis is a technique for automatic programming

applications ~\cite{gulwani2017program}:
\begin{itemize}[nolistsep,noitemsep]
    \item Data Wrangling 
    \item Graphics
    \item Code Repair
    \item Code Suggestions
    \item Modeling
    \item Superoptimization
    \item Concurrent Programming
\end{itemize}
aritra verdict: our focus is primarily modeling, with superoptimization.

Learning neurosymbolic generative models via program synthesis

Bayesian synthesis of probabilistic programs for automatic data modeling

Data-driven synthesis of full probabilistic programs

\subsection{Extra notes}

qalgozoo, QSVT

VQA, annealing, QAOA  - note we don't discuss this too much

    we focus on structured QAlgo than heuristics

Every step in AQSE can be informed by user intent to bridge the spectrum between manual and automatic.
So, you can force AQSE to generate a quantum solution for addition, but the default setting is where it just gives out a classical code when your requirement is some arithmetical operations.
Since it depends on the pipeline, that manual override can help to get a quantum solution, plug in the full pipeline, and empirically test if it performs better for real-world data.

While the proof of computational usefulness can also eithr be complexity theoretic, or by timestep statistics.

(with optional use specified resource hard constraints or soft costs).

\textbf{Review of Similar tools (merge in individual category)}

Specific to Quantum software

CQC: DisCoCat, DisCoPy, DisCoCirc, DisCoPyro: monoidal category, differentiable programming

Topos Institute: Catlab.jl based on Generalized Algebraic theories

MELVIN, AdaQuantum

computer algebra systems, string rewriting systems

More general Classical software:

HL/Beh synthesis

make dictionary with semantic ID and string
make nx graph of semantic nodes and relations (hypergraph?)
same for perception and action
